# Supplementary material for: Sample-Efficient Optimization in the Latent Space of Deep Generative Models via Weighted Retraining
Source: arXiv:2006.09191 source file (2020-10-25)
Supplement: Supplementary file 1 [file pseudocode.tex]

\section{Pseudocode of Latent Manifold Optimization with Weighted Retraining}
\label{sec:pseudocode}
\begin{algorithm}[th]
\caption{Latent Manifold Optimization {\color{blue} with Weighted Retraining} (changes highlighted in {\color{blue} blue})}
\label{alg:pseudocode}
\begin{algorithmic}
    \STATE {\bfseries Input:} Data $\D = \{\x_n\}_{n=1}^N$, query budget $B$, objective function $f(\x)$, encoder model $e_\phi(\z|\x)$, decoder model $d_\theta(\x|\z)$, predictive model $t_\psi(\z)$, {\color{blue} retraining budget $R$, weighting function $w(\x)$}
    \vspace{1mm}
    {\color{blue}\FOR{$1, \ldots, R$}
        {\color{black} \STATE Train DGM on data $\D$ {\color{blue} weighted by $\mathcal{W} = \{w(\x)\}_{\x \in \D}$} to get $\phi_*$ and $\theta_*$
        \vspace{1mm}
    	\FOR{$1, \ldots, B$\textcolor{blue}{$/R$}}
            \STATE Compute latents $\mathcal{Z} = \{\z \sim e_{\phi_*}(\z|\x)\}_{\x \in \D}$ and function values $\mathcal{V} = \{f(\x)\}_{\x \in \D}$ of $\D$
            \STATE Fit predictive model to $\mathcal{Z}$ and $\mathcal{V}$ to get $\psi_*$, and suggest new latent $\tilde{\z}$ based on $t_{\psi_*}$
    	    \STATE Obtain corresponding input $\tilde{\x} \sim d_{\theta_*}(\x|\tilde{\z})$ and update dataset $\D = \D \cup \{\tilde{\x}\}$
        \ENDFOR}
    \ENDFOR}
    \vspace{1mm}
	\STATE {\bfseries Output:} Approximate global optimizer of the objective function, $\x^* = \operatorname{arg\ max}_{\x \in \D} f(\x)$
\end{algorithmic} 
\end{algorithm}
